# Supplementary material for: Cascade IPG Observer for Underwater Robot State Estimation
Source: arXiv:2504.15235 source file (2025-04-21)
Supplement: Supplementary file 1 [file appendix.tex]

% \section*{APPENDIX}

% Revisiting the dynamic equation (Eqn \ref{eqn:dyneqn}) for the ROV, the $M$ and $C$ matrix contain effects of both rigid body dynamics $(RB)$ and hydrodynamics (added mass $A$). Hence the equation can be split as follows:
% \begin{equation}
%     M_{RB} \dot{v} + M_A \dot{v} + C_{RB} (v) v + C_A (v) v + D(v) v + g(\eta) = \tau
% \end{equation}
% From \cite{Fossen2011}, we get the rigid mody mass matrix as follows:
% \begin{equation}
%     M_{RB} = \begin{bmatrix}
%         m   & 0     & 0     & 0    & mz_g    & -my_g \\
%         m   & m     & 0     & -mz_g    & 0    & mx_g \\
%         m   & 0     & m     & my_g    & -mx_g    & 0 \\
%         0    & -mz_g    & my_g     & I_x    & -I_{xy}    & -I_{xz} \\
%         mz_g    & 0    & -mx_g     & -I_{yx}    & I_y    & -I_{yz} \\
%         -my_g    & mx_g    & 0  & -I_{zx}    & -I_{zy}    & I_z \\
%     \end{bmatrix}
% \end{equation}
% Here, $x_g$, $y_g$ and $z_g$ are the coordinates of the center of gravity of the ROV w.r.t to the geometric center of the ROV. $I_k$ is the moment of inertia along $k$ axis and the moment of inertia products are $I_{xy} = I_{yx}$, $I_{yz} = I_{zy}$ and $I_{xz} = I_{zx}$ due to symmetry. Moreover, the lateral geometric symmetry of the ROV indicates that $x_g = 0$ and $y_g = 0$. Additionally, $I_{xy} = I_{yz} = I_{xz} = 0$. Hence,
% \begin{equation}
%     M_{RB} = \begin{bmatrix}
%         m   & 0     & 0     & 0    & mz_g    & 0 \\
%         m   & m     & 0     & -mz_g    & 0    & 0 \\
%         m   & 0     & m     & 0    & 0    & 0 \\
%         0    & -mz_g    & 0     & I_x    & 0    & 0 \\
%         mz_g    & 0    & 0     & 0    & I_y    & 0 \\
%         0     & 0   & 0  & 0    & 0    & I_z \\
%     \end{bmatrix}
% \end{equation}
% In a similar fashion, the matrices $M_A$, $C_{RB}$ and $C_A$ are formulated as follows \cite{wu_6-dof_nodate}:
% \begin{align}
%     M_A&=-\left[\begin{array}{cccccc}
% X_{\dot{u}} & 0 & 0 & 0 & 0 & 0 \\
% 0 & Y_{\dot{v}} & 0 & 0 & 0 & 0 \\
% 0 & 0 & Z_{\dot{w}} & 0 & 0 & 0 \\
% 0 & 0 & 0 & K_{\dot{p}} & 0 & 0 \\
% 0 & 0 & 0 & 0 & M_{\dot{q}} & 0 \\
% 0 & 0 & 0 & 0 & 0 & N_{\dot{r}}
% \end{array}\right]\\
%     C_{R B}(v)&=\left[\begin{array}{cccccc}0 & 0 & 0 & 0 & m w & 0 \\ 0 & 0 & 0 & -m w & 0 & 0 \\ 0 & 0 & 0 & m v & -m u & 0 \\ 0 & m w & -m v & 0 & I_z r & -I_y q \\ -m w & 0 & -m u & -I_z r & 0 & I_x p \\ m v & -m u & 0 & I_y q & -I_x p & 0\end{array}\right] \\
% C_A(v)&=\left[\begin{array}{cccccc}
% 0 & 0 & 0 & 0 & z_{\dot{w}} w & 0 \\
% 0 & 0 & 0 & -z_{\dot{w}} w & 0 & -X_{\dot{u}} u \\
% 0 & 0 & 0 & -Y_{\dot{v}} v & X_{\dot{u}} u & 0 \\
% 0 & -z_{\dot{w}} w & Y_{\dot{v}} v & 0 & -N_{\dot{r}} r & M_{\dot{q}} q \\
% z_{\dot{w}} w & 0 & -X_{\dot{u}} u & N_{\dot{r}} r & 0 & -K_{\dot{p}} p \\
% -Y_{\dot{v}} v & X_{\dot{u}} u & 0 & -M_{\dot{q}} q & K_{\dot{p}} p & 0
% \end{array}\right]
% \end{align}
% The damping matrix $D \in \mathbb{R}^{6\times6}$ is computed experimentally following the method in \cite{wu_6-dof_nodate} will be used as a direct parameter in the final equation. The damping matrix is an effect of the following:
% \begin{enumerate}
%     \item Wave Drift Damping - \textit{(is neglected for underwater vehicles)}
%     \item Potential Damping - \textit{(is neglected for underwater vehicles)}
%     \item Skin Friction - linear damping taken as $D_L$ 
%     \item Vortex Shedding - quadratic damping taken as $D_{NL}$
% \end{enumerate}
% Therefore, the resultant damping term $D(\nu)$ is 
% \begin{equation}
%     D(\nu) = D_L + D_{NL}(\nu)
% \end{equation}
% Here, 
% \begin{align}
%     D_L &= -diag[X_u, Y_u, Z_u, K_p, M_p, N_p] \\
%     D_{NL}(\nu) &= -diag[X_{u|u|} |u|, Y_{v|v|} |v|, Z_{w|w|}|w|, K_{p|p|}|p|, M_{q|q|}|q|, N_{r|r|}|r|]
% \end{align}
% Hence,
% \begin{equation}
%     D(v)=-\left[\begin{array}{cccccc}X_u+X_{u|u|}|u| & 0 & 0 & 0 & 0 & 0 \\ 0 & Y_v+Y_{v|v|}|v| & 0 & 0 & 0 & 0 \\ 0 & 0 & Z_w+Z_{w|w|}|w| & 0 & 0 & 0 \\ 0 & 0 & 0 & K_p+K_{p|p|}|p| & 0 & 0 \\ 0 & 0 & 0 & 0 & M_q+M_{q|q|}|q| & 0 \\ 0 & 0 & 0 & 0 & 0 & N_r+N_{r|r|}|r|\end{array}\right]
% \end{equation}

% The restoring force vector matrix can be written as:
% \begin{equation}
%     g(\eta) = \begin{bmatrix}
%         (W-B) \sin{\theta}\\
%         -(W-B)\cos{\theta}\sin{\phi}\\
%         -(W-B)\cos{\theta}\cos{\phi}\\
%         z_g W \cos{\theta} \sin{\phi}\\
%         z_g W \sin{\theta}\\
%         0
%     \end{bmatrix}
% \end{equation}
% where $B = \rho g \nabla$ is the buoyancy force and $W = mg$ is the weight of the ROV. Here, $\rho$ is the density of water and $\nabla$ is the volume of water displaced due to the ROV. 
